# Supplementary material for: Quantum Gravitational Corrections to Electromagnetism And Backreaction
Source: arXiv:2307.02580 source file (2023-07-05)
Supplement: Supplementary file 1 [file appendix.tex]

\chapter{The Vertices}\label{appendix:vertices}

\begin{tabular}{ll}
\textit{$\bullet$ 2-Scalars-1-Photon Vertex} & \\
\parbox[c]{4cm}{
      \includegraphics[width=4cm]{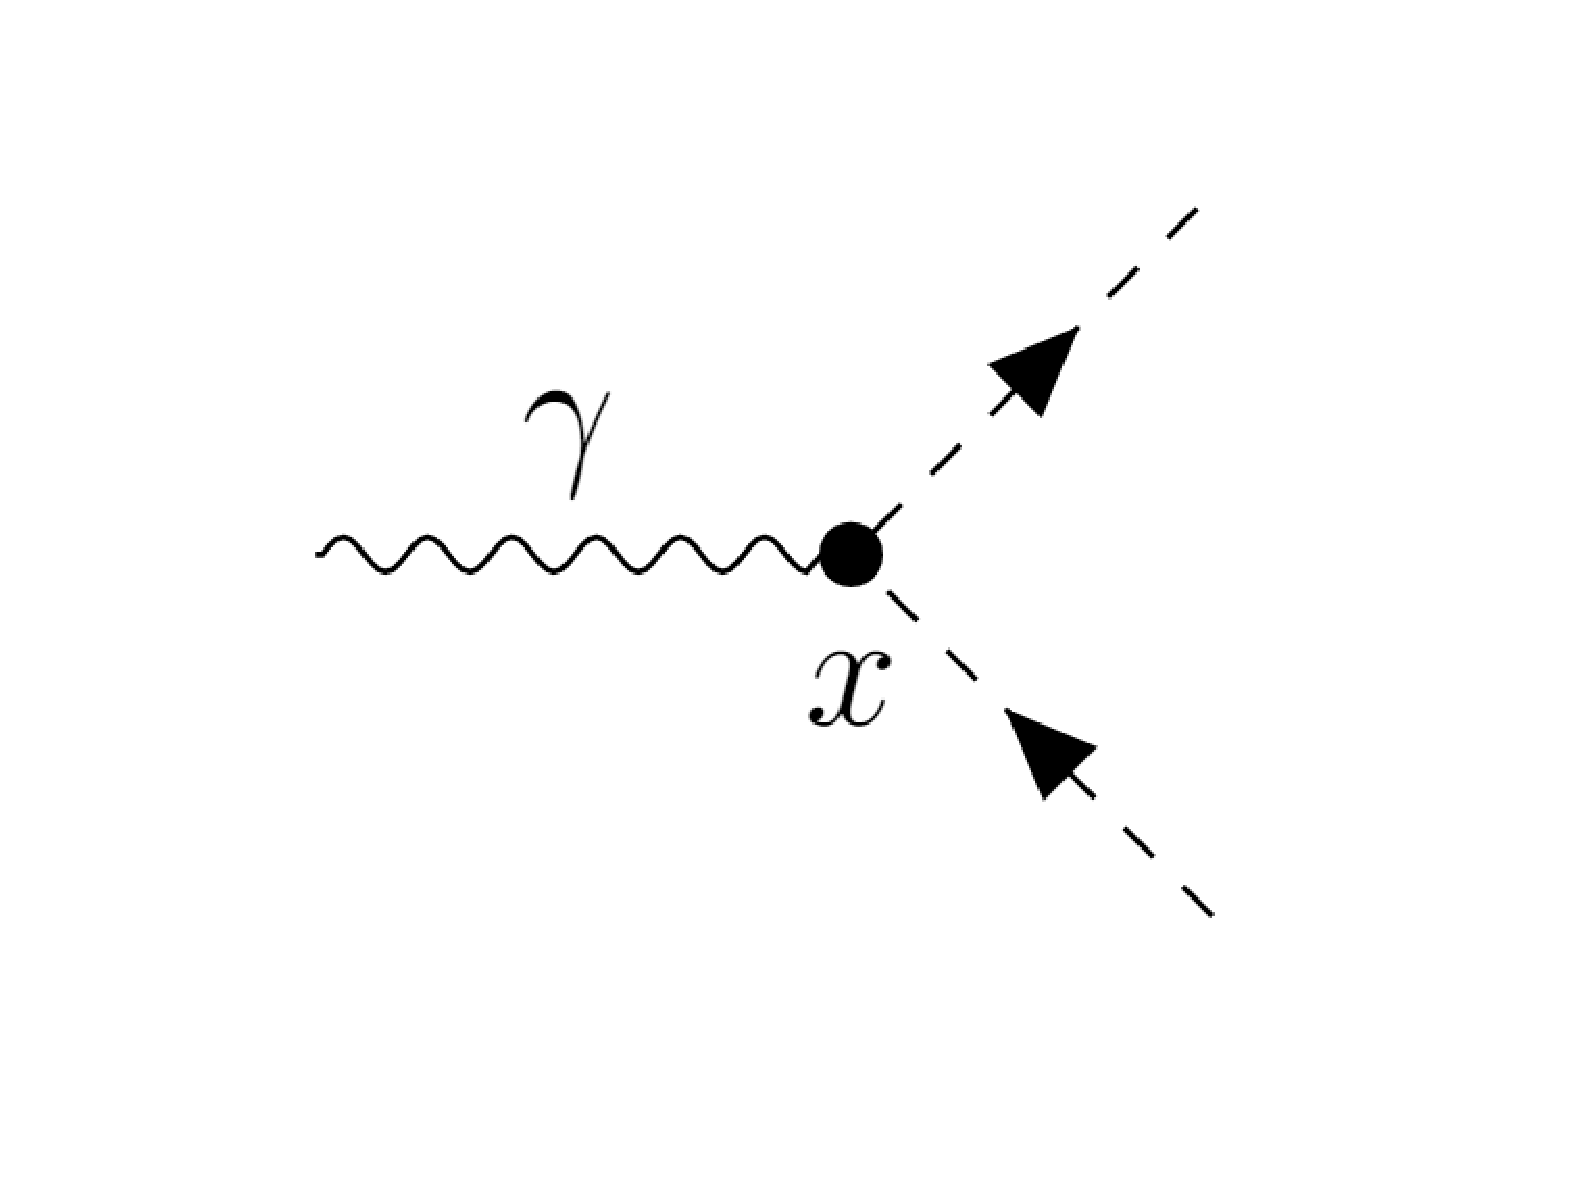}} & \parbox[l]{8.4cm}{\begin{equation} =e(\partial_x\downarrow-\partial_x\uparrow)^\gamma 
      \end{equation}}\\[1cm]
   \textit{$\bullet$ 2-Scalars-2-Photon Vertex}& \\
   \parbox[c]{4cm}{\includegraphics[width=4cm]{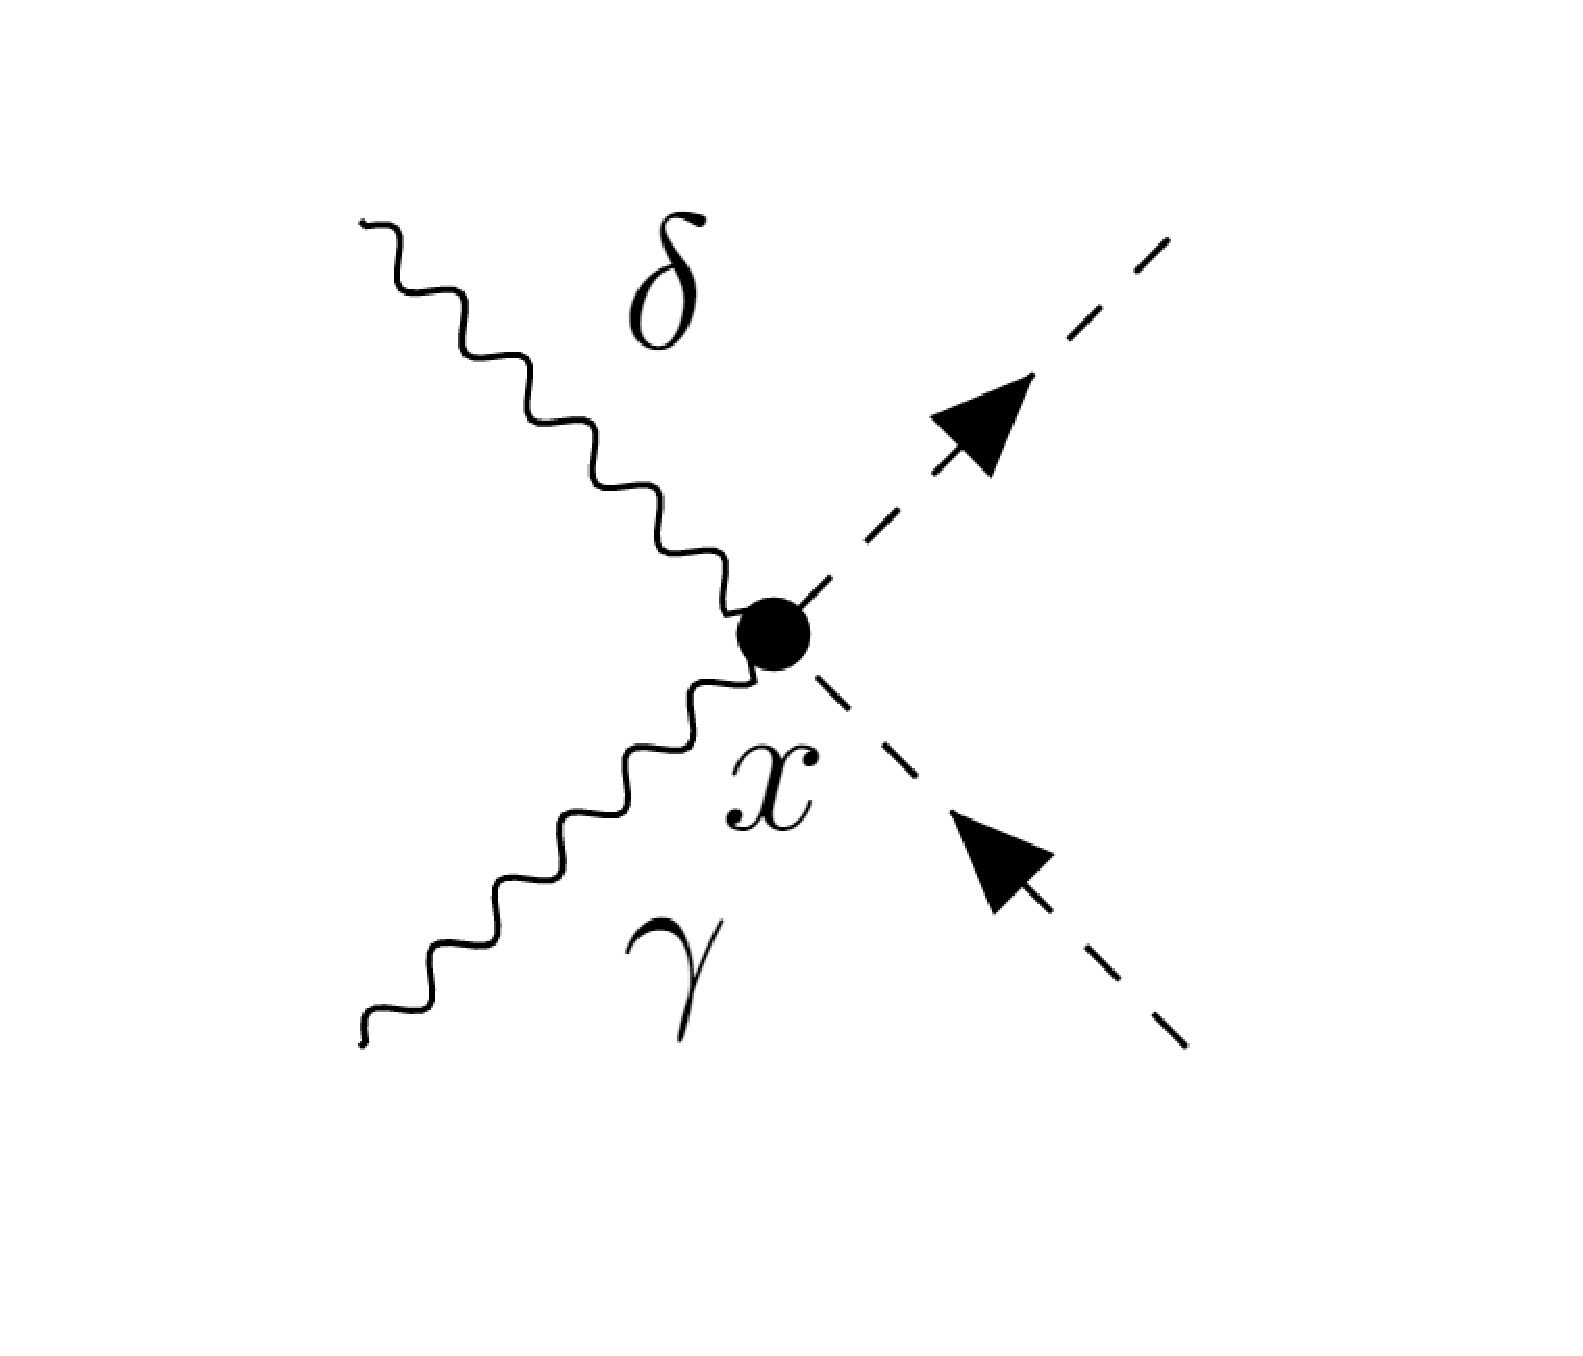}} & \parbox[l]{8.4cm}{\begin{equation}=-2ie^2\eta^{\gamma\delta}
   \end{equation}}\\[1cm]
   \textit{$\bullet$ 2-Scalars-1-Graviton Vertex} & \\
   \parbox[c]{4cm}{\includegraphics[width=4cm]{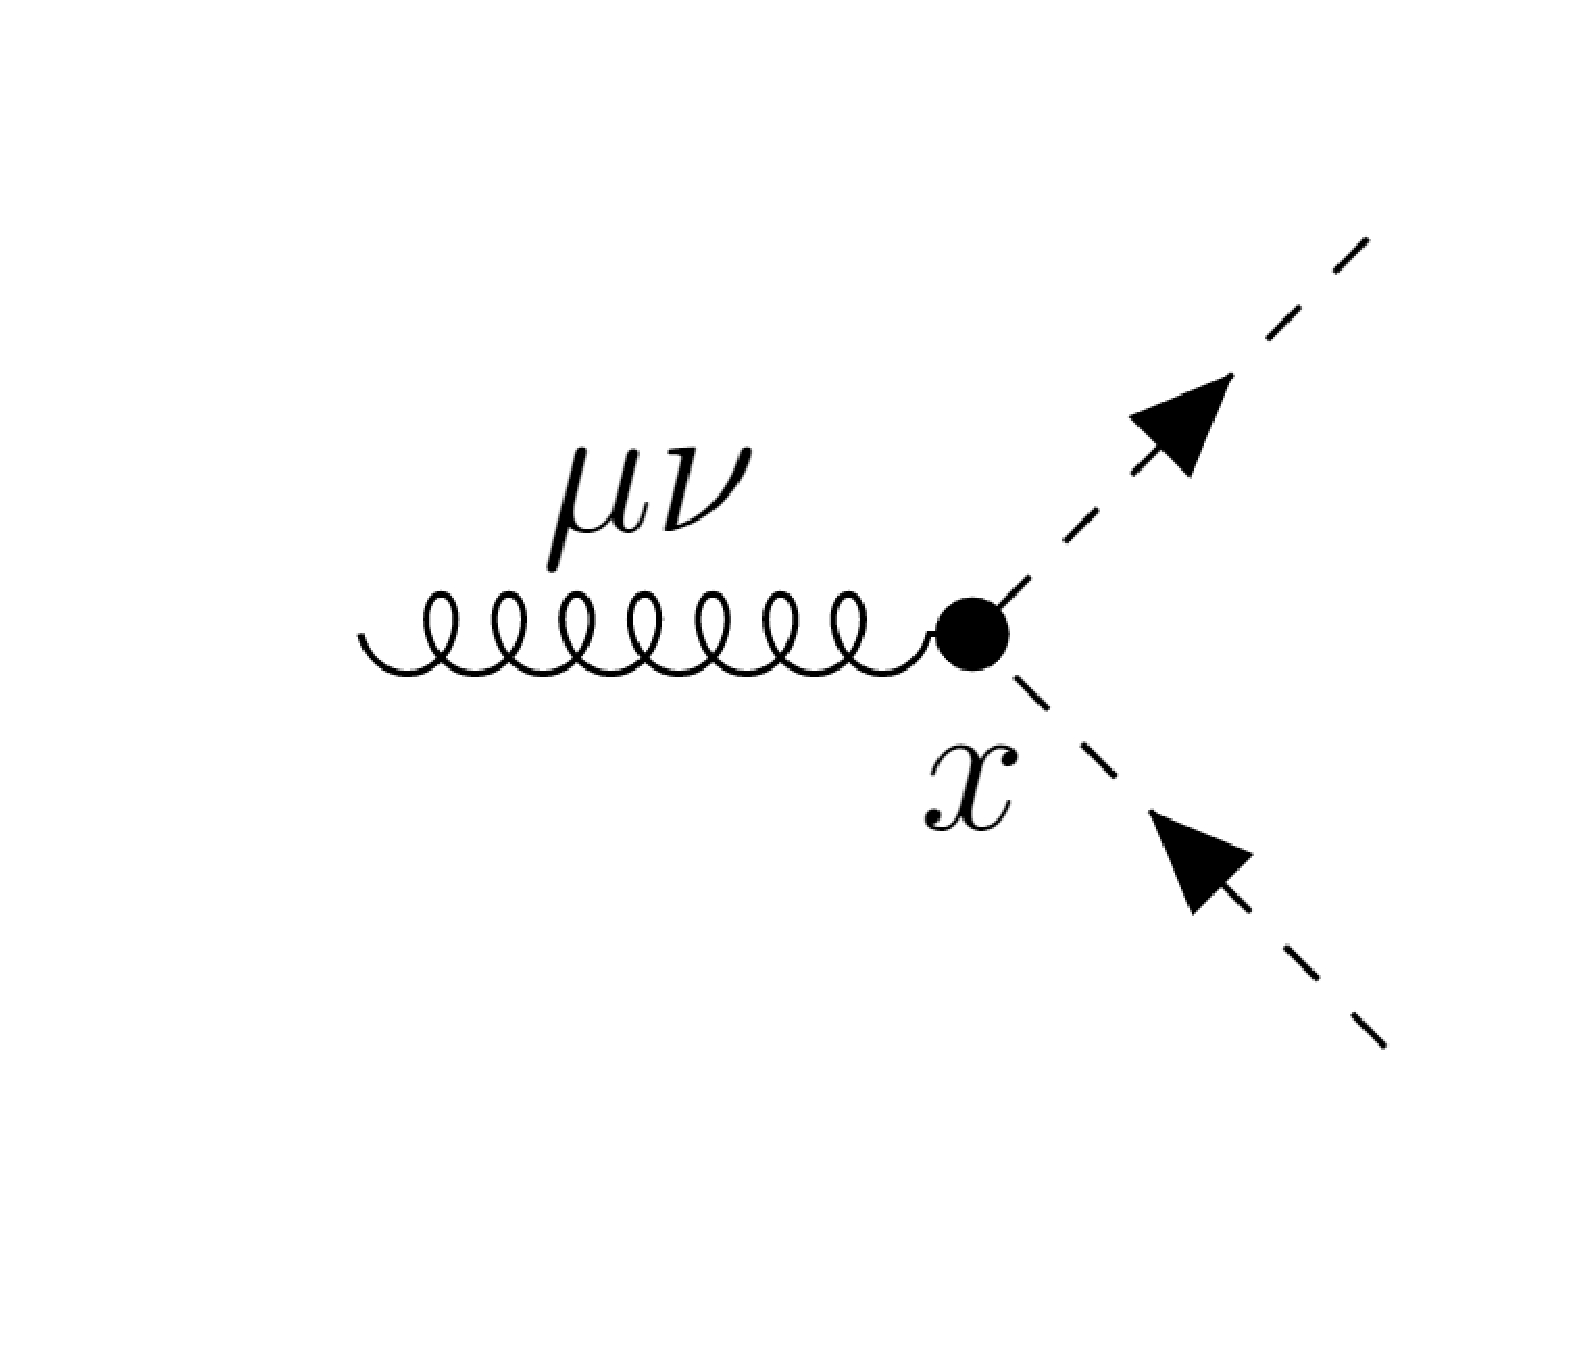}} &  \parbox[l]{8.4cm}{\begin{equation}\begin{split}
=\frac{i\kappa}{2}[&\partial_x^\mu\uparrow\partial^\nu_x\downarrow+\partial^\nu_x\uparrow\partial^\mu_x\downarrow\\
&- \eta^{\mu\nu}(\partial_x\uparrow\cdot\partial_x\downarrow+m^2)]
\end{split}
 \end{equation}}\\[1cm]
   \textit{$\bullet$ 2-Scalars-1-Photon-1-Graviton Vertex} & \\
   \parbox[c]{4cm}{\includegraphics[width=4cm]{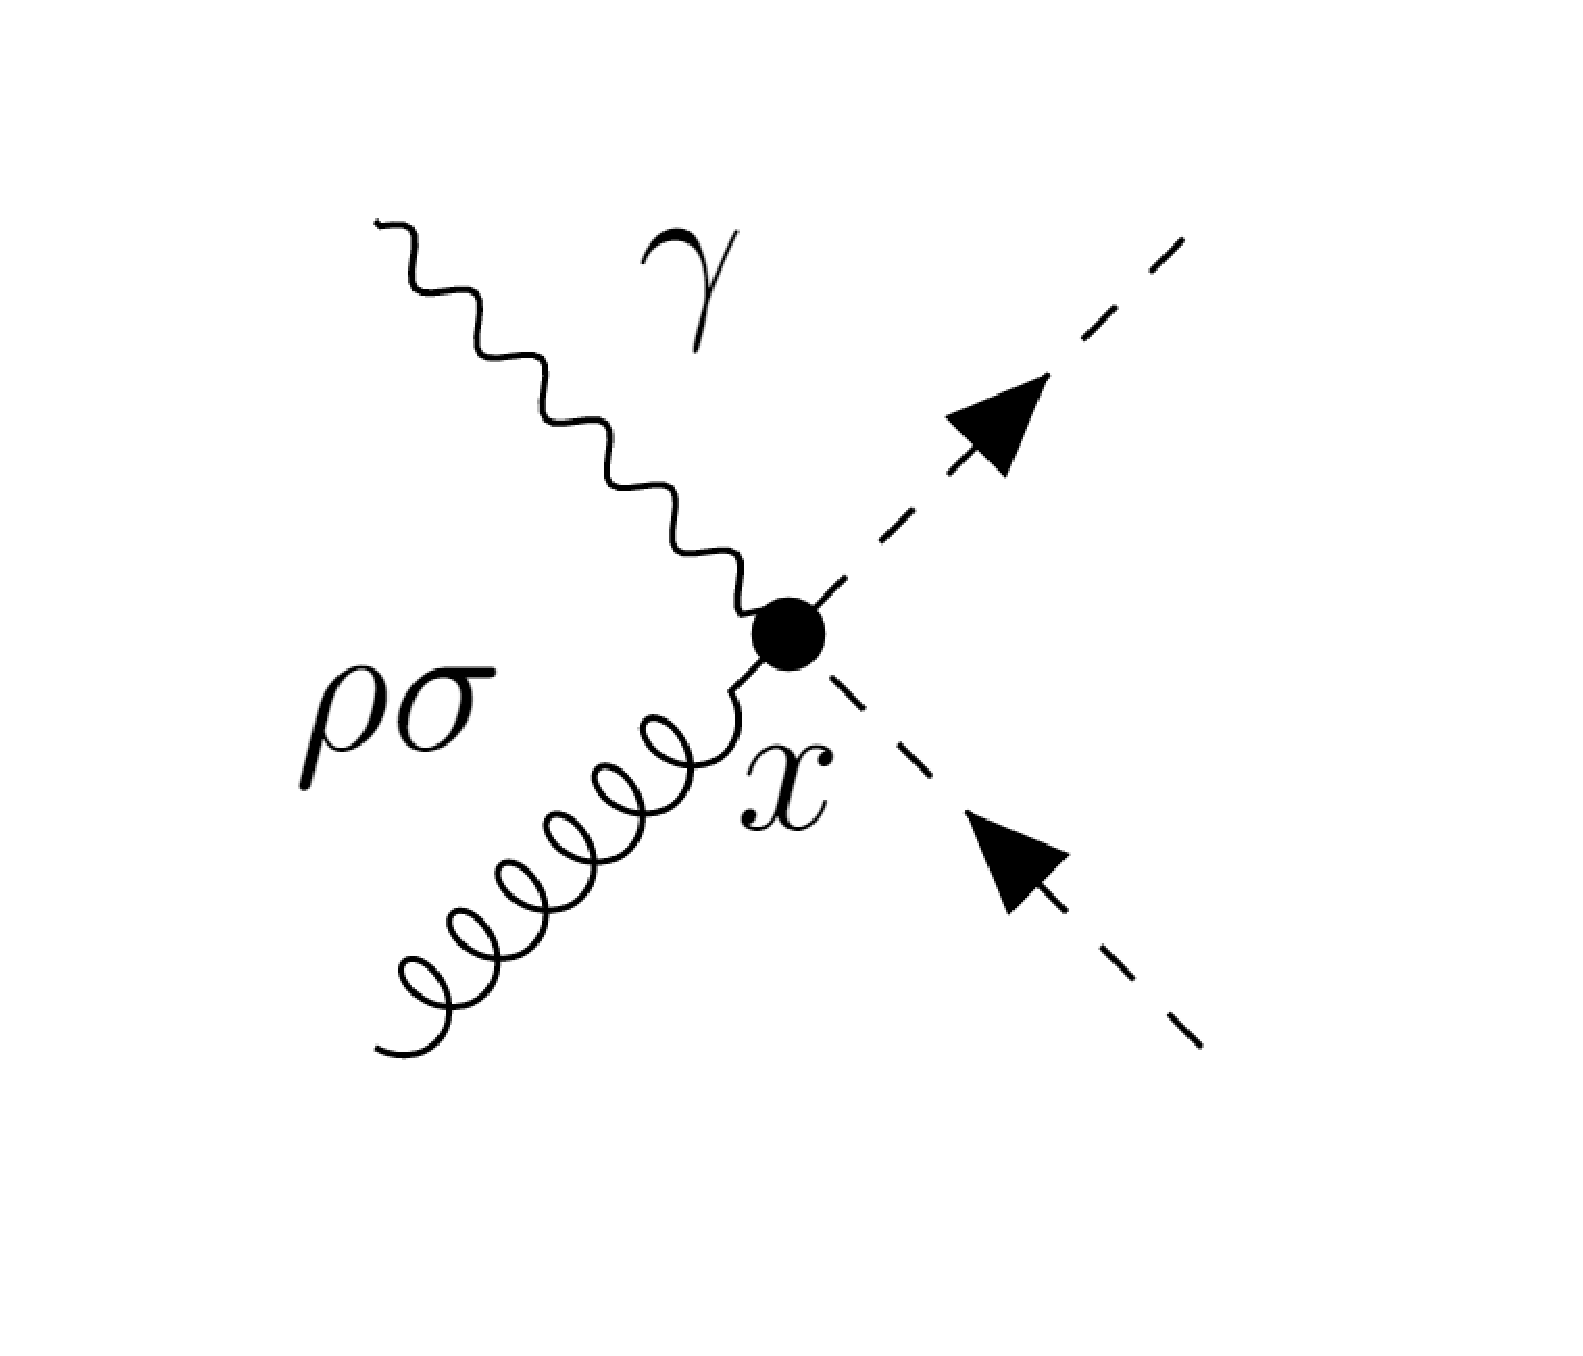}} & \parbox[l]{8.4cm}{\begin{equation}\begin{split}
   =\frac{e\kappa}{2}[&\eta^{\gamma\rho}\eta^{\alpha\sigma}+\eta^{\gamma\sigma}\eta^{\alpha\rho}-\eta^{\rho\sigma}\eta^{\alpha\gamma}]\\
   &\times(\partial_x\uparrow-\partial_x\downarrow)_\alpha
   \end{split}
   \end{equation}}\\[1cm]
   \textit{$\bullet$ 2-Photon-1-Graviton Vertex} & \\
   \parbox[c]{4cm}{\includegraphics[width=4cm]{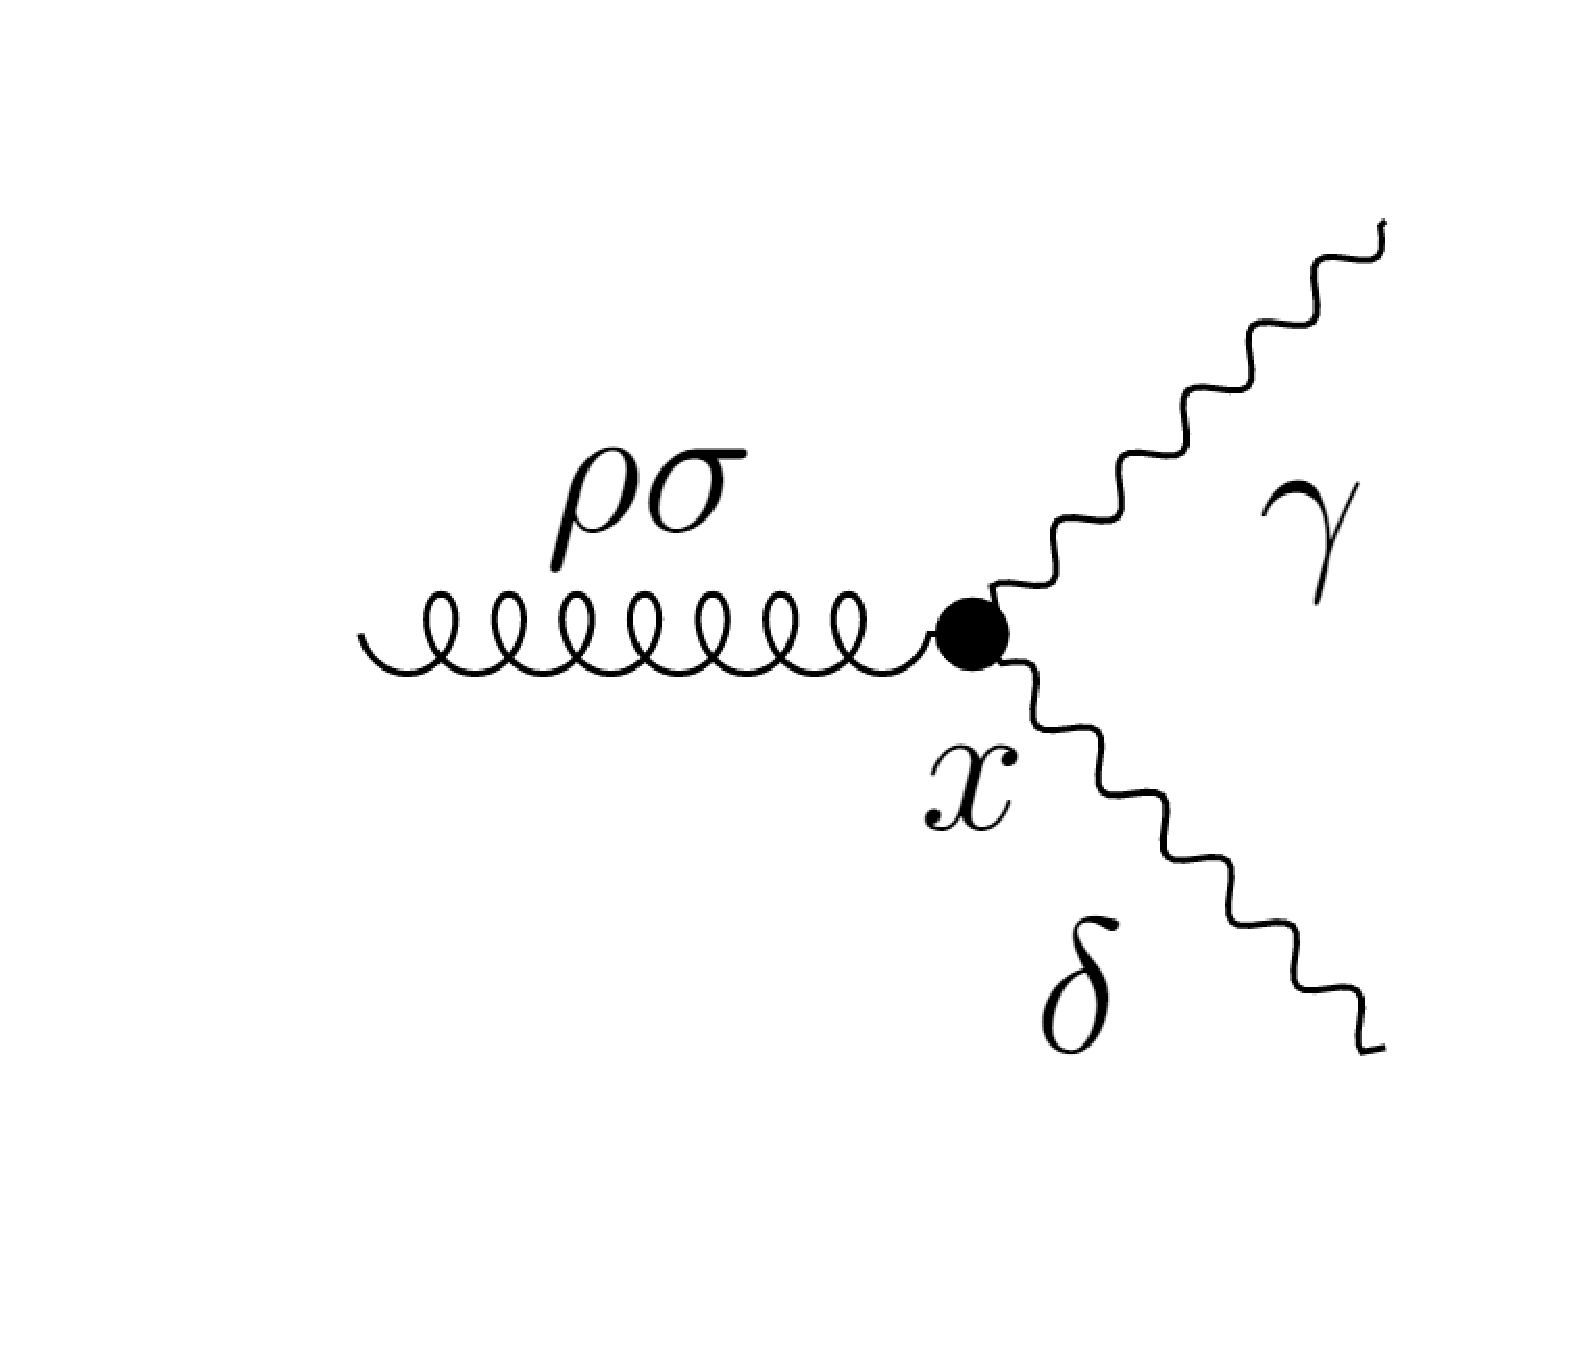}} & \parbox[l]{8.4cm}{\begin{equation}\label{vert_2p1g}\begin{split}&=-i\kappa V^{\gamma\delta\alpha\tau\rho\sigma} \partial_\alpha\uparrow\partial_\tau\downarrow\\
   &\text{where,}\\
   &\ V^{\gamma\delta\alpha\tau\rho\sigma}= \eta^{\rho\sigma}\eta^{\alpha[\tau}\eta^{\delta]\gamma}+4\eta^{\rho)[\gamma}\eta^{\alpha][\delta}\eta^{\tau](\sigma}\end{split}\end{equation}}
\end{tabular}

\chapter{Propagators}\label{appendix:propagators}

The massless scalar propagator $i\Delta(x;x')$ obeys the equation,
\begin{equation}\label{eq:equation_massless}
    \partial^2 i \Delta(x;x') = i \delta^D(x \!-\! x') \; .
\end{equation}
Even in $D$ spacetime dimensions it has a simple expression in terms of Lorentz 
interval $\Delta x^2(x;x')$,
\begin{equation}\label{massless_scalar_prop}
    i\Delta(x;x') = \frac{\Gamma(\frac{D}{2}-1)}{4\pi^{D/2}}
    \left(\frac{1}{\Delta x^2}\right)^{\frac{D}2-1} \; , 
\end{equation}
where we define,
\begin{equation}
    \Delta x^2(x;x') \equiv ||\Vec{x}-\Vec{x}'||^2 - \left(|t-t'|-i\varepsilon\right)^2 \; .
\end{equation}
The massive scalar propagator $i\Delta_m(x;x')$ obeys the equation,
\begin{equation}\label{massive_scalar_prop}
    (\partial^2 - m^2) i \Delta_m(x;x') = i \delta^D(x \!-\! x') \; .
\end{equation}
It can be written in terms of Bessel functions but the expression itself is not 
necessary for purposes. It turns out that we can always eliminate $i\Delta_{m}(x;x')$,
either with the propagator equation (\ref{massive_scalar_prop}) or by recourse
to one of the Donoghue Identities given in Appendix \ref{appendix:donoghue}.

The photon field also requires gauge fixing. The most general Poincar\'e invariant 
gauge fixing functional depends upon an arbitrary parameter $c$,
\begin{equation}
    \mathcal{L}_{\text{EMfix}} = -\frac{1}{2c} (\partial^\mu A_\mu)^2 \; .
\end{equation}
The associated propagator can be expressed using the massless scalar propagator 
(\ref{massless_scalar_prop}),
\begin{equation}
    i[_\rho\Delta_\sigma](x;x') = \left[ \eta_{\rho\sigma} + (c\!-\!1) 
    \frac{\partial_{\rho} \partial_{\sigma}}{\partial^2} \right] i\Delta(x;x') \; .
\end{equation}
The longitudinal term proportional to $c-1$ presumably drops out due to current
conservation but we shall simply adopt the $c=1$ Feynman gauge that Bjerrum-Bohr 
employed \cite{Bjerrum-Bohr:2002aqa},
\begin{equation}
    i[_\rho\Delta_\sigma](x;x') = \eta_{\rho\sigma} i \Delta(x;x') \; .
\end{equation}

The most general Poincar\'e invariant gauge fixing function (\ref{gauge}) depends 
on two parameters $a$ and $b \neq 2$ (for $b = 2$ the gauge fixing functional 
degenerates to the square of a linearized Ricci scalar). To simplify the analysis
we work only to first order in the perturbations $a = 1 + \delta a$ and $b = 1 + 
\delta b$,
\begin{equation}\label{eq:graviton_prop}
\begin{split}
    i[_{\mu\nu}\Delta_{\rho\sigma}](x;x') = \Biggl[ 2 \eta_{\mu(\rho} \eta_{\sigma)\nu}
    -\frac{2 \eta_{\mu\nu} \eta_{\rho\sigma}}{D \!-\! 2} & + \frac{4 \delta a 
    \partial_{(\mu}\eta_{\nu)(\rho}\partial_{\sigma)}}{\partial^2} \\
    & -2 \delta b \left(\eta_{\mu\nu} \frac{\partial_{\rho} \partial_{\sigma}}{\partial^2}
    + \eta_{\rho\sigma} \frac{\partial_{\mu}\partial_{\nu}}{\partial^2} \right)\Biggr]
    i\Delta(x;x') \; .
    \end{split}
\end{equation}

\chapter{The Donoghue Identities}\label{appendix:donoghue}

What we term the ``Donoghue Identities'' are not equalities but rather relations
for extracting the nonlocal and nonanalytic parts of amplitudes which can contribute
to long range forces. As originally derived by Donoghue and collaborators
\cite{Donoghue:1993eb,Donoghue:1994dn,Donoghue:1996mt}, they included nonlinear
classical effects as well as quantum effects, but we have retained only the parts
relevant for quantum effects. When expressed in position space these relations all
have the effect of degenerating massive propagators to delta functions. We required
six such relations, of which the final two (those involving factors of $1/\partial^2$) 
were derived by us for this project:
 \begin{itemize}
        \item This concerns 3-point diagrams with no derivatives acting on propagators,
        \begin{equation}\label{eq:3pt}
            i\Delta_m(x;y) i\Delta(x;x') i\Delta(y;x') \longrightarrow 
            \frac{i \delta^D(x \!-\!y)}{2m^2} [i\Delta(x;x')]^2 \; .
        \end{equation}
        \item This concerns 3-point diagrams with a derivative acting on a massless 
        propagator,
        \begin{equation}\label{eq:3pt_derivative}
            \left[\partial_x^{\mu} i\Delta(x;x') \right] i\Delta_m(x;y)
            i\Delta(y;x') \longrightarrow -\partial_{x}^{\mu} 
            \left[\frac{i\delta^D(x \!-\! y)}{2m^2} [i\Delta(x;x')]^2\right] \; .
        \end{equation}
        \item This concerns 3-point diagrams with two derivatives acting on a 
        massless propagator,
        \begin{equation}\label{eq:3pt_2derivative}
            \begin{split}
                \left[\partial_{x}^{\mu} \partial_{x}^{\nu} i\Delta(x;x') \right]
                i\Delta_m(x;y) & \Delta(y;x') \longrightarrow \Bigl\{\partial_{x}^{\mu}
                \partial_{x}^{\nu} \frac{(\partial_{x} \!+\! \partial_{y})^2}{2m^2}
                -\frac{1}{2} \Bigl(\partial_{x}^{\mu} (\partial_{x} \!+\! \partial_{y})^{\nu} \\
                & + \partial_{x}^{\nu} (\partial_{x} \!+\! \partial_{y})^{\mu} \Bigr)
                - \frac{1}{4} \eta^{\mu\nu} (\partial_{x} \!+\! \partial_{y})^2\Bigr\}
                \left[\frac{i\delta^D(x \!-\!y)}{2m^2} [i\Delta(x;x')]^2\right] \; .
            \end{split}
        \end{equation}
        \item These concern 4-point diagrams with no derivatives acting on the propagators. 
        The first is relevant to the box diagrams as shown on the upper part of Figure~\ref{fig:box}. 
        The second is relevant to the cross diagrams as shown on the lower part of Figure~\ref{fig:box},
        \begin{equation}\label{eq:box_dono}
            \begin{split}
                m^2 (\partial_{x} \!+\! \partial_{y})^2 & \left[i\Delta_m(x;y) i\Delta(y;y')
                i\Delta_m(y';x') i\Delta(x';x)\right] \\
                & \longrightarrow \left(1-\frac{\partial_{x} \!\cdot\! \partial_{x'} \!-\! m^2}{3m^2}
                \right)[i\Delta(x;x')]^2 \delta^D(x\!-\!y) \delta^D(x' \!-\!y') \; , \\
                 m^2 (\partial_{x} \!+\! \partial_{y})^2 & \left[i\Delta_m(x;y) i\Delta(y;x')
                 i\Delta_m(x';y') i\Delta(y';x)\right] \\
                 & \longrightarrow \left(-1 \!+\! \frac{\partial_{x}\!\cdot\! \partial_{y'} \!-\! m^2}{3m^2}
                 \right)[i\Delta(x;x')]^2 \delta^D(x\!-\!y) \delta^D(x'\!-\!y') \; .
            \end{split}
        \end{equation}
        \item This concerns 3-point diagrams with a derivative and an inverse Laplacian 
        on a massless propagator,
        \begin{equation}\label{eq:new_dono_1}
            \begin{split}
                i\Delta_m(x;y) & i\Delta(x;x') \frac{\partial^\mu}{\partial^2} \Delta(y;x') \\
                & \longrightarrow \frac{1}{m^2} \Bigl[\frac{(\partial_{x} \!+\! \partial_{y})^{\mu}}{8}
                - \frac{\partial_x^{mu}}{2} + \frac{1}{3m^2} \partial_{x}^{\mu} 
                (\partial_{x} \!+\! \partial_{y})^2 \Bigr] \left[\frac{i\delta^D(x\!-\!y)}{2m^2}
                [i\Delta(x;x')]^2 \right] .
            \end{split}
        \end{equation}
        \item This concerns 3-point diagrams with two derivatives and an inverse Laplacian 
        on a massless propagator,
        \begin{equation}\label{eq:new_dono_2}
            \begin{split}
                i\Delta_m(x;y) i\Delta(x;x')&\frac{\partial^\mu\partial^\nu}{\partial^2}\Delta(y;x')\\
                &\longrightarrow\Bigl[\frac{1}{2}\eta^{\mu\nu}-\frac{1}{m^2}\partial_{x}^\mu\partial_x^\nu+\frac{1}{6m^2}\eta_{\mu\nu}(\partial_x+\partial_y)^2+\frac{1}{2m^2}\Bigl(\partial_{x}^\mu(\partial_x+\partial_y)^\nu\\
                &+\partial_{x}^\nu(\partial_x+\partial_y)^\mu\Bigr)-\frac{2}{3m^4}(\partial_x+\partial_y)^2\partial_x^\mu\partial_x^\nu\Bigr]\left[\frac{i\delta^D(x\!-\!y)}{2m^2}[i\Delta(x;x')]^2\right] .
            \end{split}
        \end{equation}
    \end{itemize}
